# Supplementary material for: Topological Characterization of Rigid-Nonrigid Transition across the Frenkel Line
Source: arXiv:1807.02761 source file (2018-10-14)
Supplement: Supplementary file 1 [file Supporting_Information_for_Topological_Characterization_of_Rigid_Nonrigid_Transition_across_the_Frenkel_Line.pdf]

# Supporting Information for Topological Characterization of Rigid-Nonrigid Transition across the Frenkel Line

Tae Jun Yoon,[1] Min Young Ha,[1] Emanuel A. Lazar,[2] Won Bo Lee,[1, a)] and Youn-Woo Lee[1, b)]
[1)] *School of Chemical and Biological Engineering, Institute of Chemical Processes, Seoul National University, Seoul 08826, Republic of Korea*
[2)] *Materials Science and Engineering, University of Pennsylvania, Philadelphia, PA 19104*

(Dated: 8 October 2018)

This Supporting Information includes the calculation procedures and numerical results used in the main article. In Section I, we explain the calculation procedures. In section II, some additional results relevant to the main article are described.

## I. CALCULATION DETAILS

### A. Estimation of the critical point

The critical point of 2,000 argon molecules modeled with a shifted and truncated Lennard-Jones (LJ) potential with a cutoff radius of 15.0 Åwas obtained based on the flat top proposal[1]. The flat top proposal states that the first and the second derivatives of the density to the pressure become zero at the critical point.

$$\left(\frac{\partial \rho}{\partial p}\right)_T = \left(\frac{\partial^2 \rho}{\partial p^2}\right)_T = 0 \tag{S1}$$

To obtain the pressure-density relation, NVT simulations were performed at $T = 150 - 170K$ and $\rho = 150 - 950\mathrm{kg/m}^3$. The timestep was 0.004ps. The systems were equilibrated for 100,000 steps. The pressure data were cumulatively averaged every step during the production run (1,000,000 steps). Cubic equations were used to fit the pressure-density data ($R^2 > 0.99$). The inflection point of the cubic equations were calculated, and the inflection point where the rigidity becomes zero was calculated by linear interpolation. By obtaining the critical density and temperature, the critical pressure was obtained by using the fitted equations. The critical point of argon obtained in this manner was $\rho_c = 471.45$ kg/m$^3$, $T_c = 159.14$ K, and $p_c = 60.87$ bar.

### B. Molecular Dynamics (MD) simulations

Canonical Molecular Dynamics (MD) simulations were performed to obtain the configurations of supercritical argon[2]. The interatomic potential of argon molecules was modeled with the Lennard-Jones (LJ) potential ($\sigma_{lj} =$ 3.405 Å and $\epsilon_{lj} = 0.238$ kcal/mol). The potential was shifted and truncated at the cutoff radius of $r_{cut} = 15.0$ Å. The critical point of argon ($\rho_c = 471.45$ kg/m$^3$, $T_c =$ 159.14 K, and $p_c = 60.87$ bar) was estimated based on the flat top proposal[1] (see the Supporting Information for the detailed procedure to obtain the critical point). After the estimation of the critical point, NVT simulations with periodic boundary conditions were performed at $T_r = T/T_c = 1.0 - 70.0$. The timesteps of simulations were 0.004 ps at $T_r = 1.0$ and 5.0, and 0.002 ps for higher temperatures. The systems were equilibrated for 10,000 steps, and the configurations of supercritical argon were obtained every 1,000 step during 500,000 steps of the production run.

### C. Generation of the configurations at the dynamic limits

Fifty configurations of the ideal gas state of 500,000 atoms were obtained by using (pseudo)random number generators. Fifty configurations of the maximally random jammed (MRJ) state were generated by performing the event-driven molecular dynamics (EDMD) simulations[3] with 500,000 hard sphere particles in conjunction with the Lubachevsky-Stillinger compression algorithm[4]. In this algorithm, an initial configuration of atoms randomly distributed in a simulation box is first generated. The diameter of the atoms is increased so that the molecules become close to each other until the system density reaches the target density. After the system density becomes the target density, the system size is rescaled so that the diameter of the grown atoms becomes equal to their initial diameter. The target density was chosen $\phi = 0.635$, which is close to the theoretical maximum packing fraction ($\phi \sim 0.64$)[5] that a monodisperse randomly distributed spherical particles can reach.

### D. Topological characterization

VoroTop[6], an open-source software that characterizes three-dimensional atomic system based on the topological framework for local structure analysis, was used to obtain the list of the Weinberg vectors. Tutte embedding was used to draw Schlegel diagrams[7].

[a)] Electronic mail: wblee@snu.ac.kr
[b)] Electronic mail: ywlee@snu.ac.kr

### E. Cluster structure analysis

A clustering algorithm proposed by Stoll[8] was used for (1) counting the number of independent solid-like clusters and (2) determining whether a cluster is infinite or not. Here, the infinite cluster is defined as an assembly of molecules that are spanning throughout the system considering the periodic boundary condition. That is, some of its molecules that are placed at the periphery of the simulation box in opposite direction are connected with each other when the cluster size is infinite. The clustering algorithm by Stoll consists of three stages. In the first stage, solid-like molecules are clustered if and only if they share a Voronoi face with each other without a consideration of the periodic boundary conditions. In the second stage, the algorithm tests whether a solid-like molecule at the periphery of the simulation box share a face with another in the opposite direction. If those particles are Voronoi nearest neighbors, the algorithm determines that the cluster is infinite. After the infinity test, the algorithm merges the independent clusters considering the periodic boundary conditions.

### F. Finite-size effect on the classification results

To check the influence of the system size on the classification results, we conducted additional Molecular Dynamics (MD) simulations with $N = 1,000$ and $N = 8,000$ molecules at $T_r = 1.0$ and those with $N = 4,000$ and $N = 8,000$ molecules at $T_r = 10.0$.

### G. Finite-size scaling analysis

The finite-size scaling analysis on the percolation of solid-like structures across the Frenkel line was performed to estimate the percolation threshold and the correlation length exponent $\nu$. In this procedure, we initially estimated the percolation threshold based on the sigmoidal equation in the main article. The MD simulations were then performed with $N = 500, 1,000, 2,000, 4,000\ 8,000$, and $16,000$ molecules at $T_r = 1.0$ and $N = 1,000, 2,000, 4,000\ 8,000$, and $16,000$ at $T_r = 10.0$ near the estimated percolation threshold. The probability of finding an infinite cluster ($p_{inf}$) was calculated based on the algorithm proposed by Stoll. The average percolation concentration ($\Pi^{av}_{solid}$), which is defined as the fraction of solid-like molecules where the spanning cluster appears first time, was then computed as:

$$\Pi^{av}_{solid} = \int_0^1 \Pi_{solid} \left( \frac{dp_{inf}}{d\Pi_{solid}} \right) dp_{inf} \qquad \text{(S2)}$$

The derivative of $p_{inf}$ with respect to $\Pi_{solid}$ was obtained by fitting the following sigmoidal equation to the $p_{inf}$ data.

$$p_{inf} = (1 + \exp(a\Pi_{solid} + b))^c \qquad \text{(S3)}$$

TABLE S1. The coefficients estimated by fitting the sigmoid equation [Eqn. (S3)] to the probability of finding an infinite cluster in a configuration.

| $N$ | a | b | c |
|---|---|---|---|
| 500 | -12.73 | 0.000 | -6.599 |
| 1,000 | -16.65 | 0.5109 | -5.591 |
| 2,000 | -23.38 | 2.344 | -2.490 |
| 4,000 | -33.56 | 4.352 | -1.439 |
| 8,000 | -46.40 | 6.262 | -1.222 |
| 16,000 | -55.43 | 7.172 | -1.336 |

where $a$, $b$, and $c$ are the fitting parameters.

According to the percolation theory[9], the correlation length exponent $\nu$ can be obtained from the following relation.

$$\Delta \propto L^{-1/\nu} \qquad \text{(S4)}$$

where $\Delta$ is the width of the transition region in which $p_{inf}$ changes from zero to one, and $L$ is the system size. Here, we used the cube root of the number of molecules as $L$ following the method of Jerauld et al[10]. $\Delta$ is obtained by

$$\Delta^2 = \int_0^1 (\Pi_{solid} - \Pi^{av}_{solid})^2 \left( \frac{dp_{inf}}{d\Pi_{solid}} \right) d\Pi_{solid} \qquad \text{(S5)}$$

Hence, $\Delta$ is the root mean square deviation of the thresholds from their average value. Since the difference between the effective percolation threshold and the percolation threshold in an infinite system also follows the power law ($\Pi^{av}_{solid} - \Pi^{c}_{solid} \propto L^{-1/\nu}$), the percolation threshold can be obtained by plotting $\Pi^{av}_{solid}$ versus the width $\Delta$ and finding the intercept $\Pi^{c}_{solid}$ at $\Delta = 0$.

$$\Pi^{av}_{solid} - \Pi^{c}_{solid} \propto \Delta \qquad \text{(S6)}$$

## II. CALCULATION RESULTS

### A. The influence of the system size on the classification results

The influence of the system size on the classification results was negligible (Figure S1a). Hence, this result demonstrates the robustness of the classification method.

### B. Finite-size scaling analysis

Table S1 shows the fitting parameters $a$, $b$, and $c$ of Eqn. (S3). The coefficients of determination were always higher than 0.99 ($R^2 > 0.99$). Figure S1b shows the power-law relation between $L$ and the transition width $\Delta$. From the power-law fitting result, the correlation length exponent was estimated as $\nu = 0.9030 \pm 0.0319$. Then, $\Pi^{c}_{solid}$ was estimated from Eqn. (S6) as $0.1159 \pm 0.0081$.

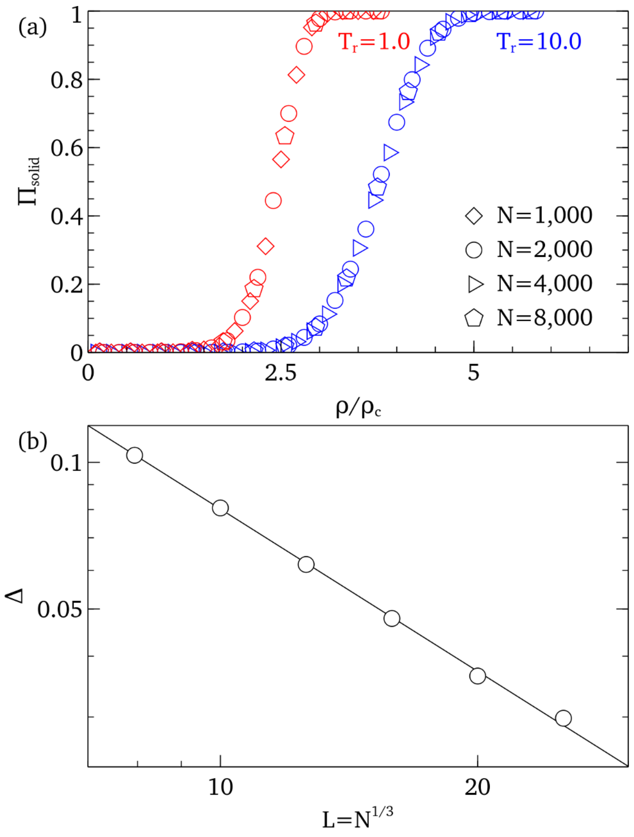


FIG. S1. (a) The system size effect on the classification results at $T_r = 1.0$ and $T_r = 10.0$. No considerable finite-size effect was observed. (b) The power-law fitting ($\Delta \sim L^{-1/\nu}$) of the system size to the transition width $\Delta$. The correlation length exponent $\nu$ was obtained as $\nu = 0.9030 \pm 0.0319$

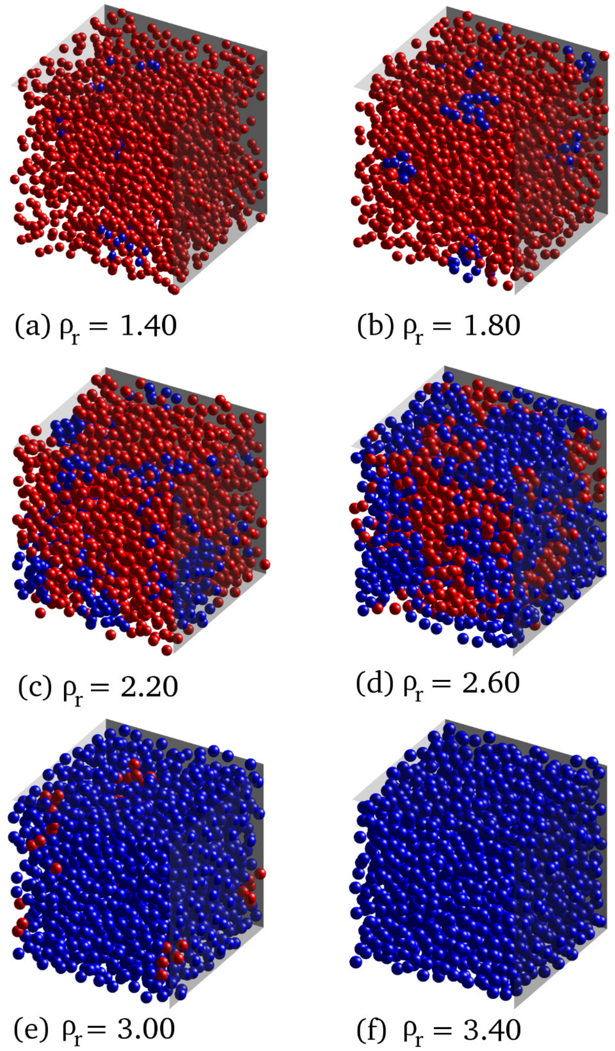


FIG. S2. Configurations of gas-like and solid-like argon molecules at $T_r = 1.0$. The number of molecules in a system was 2,000. As the density increases, the solid-like clusters (blue spheres) percolate throughout the system. Gas-like and solid-like molecules are denoted as red and blue ones, respectively.

### C. The fraction of solid-like molecules

Table S2 shows the fraction of solid-like molecules calculated from the topological classification method. They were well fitted to the sigmoidal equation [Eqn. (2) in the article].

### D. Demonstration of the structural crossover in rigid liquid region

Figure S2 shows the configurations of gas-like and solid-like argon molecules obtained from the classification algorithm.

### E. Topological information

Figure S3 and S4 show the Schlegel diagrams of the 24 most frequently observed Voronoi cells in the ideal gas and the maximally random jammed state. Compared to the ideal gas, the Voronoi cells of the MRJ state are more symmetric. Tables S3 and S4 show the Weinberg vectors and the observation frequencies of the frequently observed Voronoi cell types in the ideal gas and the MRJ state. As stated in the article, the observation frequency of the most frequently observed type in the MRJ state (3.485 %) was higher than that in the ideal gas (0.274 %) by a factor of a ten. In contrast, the observation frequency of the most scarcely observed type in the MRJ state was lower that in the ideal gas. Hence, 74,433 types of the Voronoi cells among 325,399 types observed in the MRJ state had higher observation frequencies in the MRJ state than the ideal gas.

[1] Heyes, D. The Lennard-Jones Fluid in the Liquid-Vapour Critical Region. *CMST* **2015**, *21*, 169-179.
[2] Plimpton, S. Fast Parallel Algorithms for Short-Range Molecular Dynamics. *J. Comput. Phys.* **117**, *1995*, 1-19.

TABLE S2. Dependence of the fraction of solid-like molecules on the thermodynami conditions

| | $\Pi_{solid}$ | | | | | |
|---|---|---|---|---|---|---|
| $\rho_r$ | $T_r = 1.0$ | $T_r = 5.0$ | $T_r = 10.0$ | $T_r = 30.0$ | $T_r = 50.0$ | $T_r = 70.0$ |
| 0.20 | 0.0000 | 0.0000 | 0.0000 | 0.0000 | 0.0000 | 0.0000 |
| 0.40 | 0.0000 | 0.0000 | 0.0000 | 0.0000 | 0.0000 | 0.0000 |
| 0.60 | 0.0000 | 0.0000 | 0.0000 | 0.0000 | 0.0000 | 0.0000 |
| 0.80 | 0.0001 | 0.0000 | 0.0000 | 0.0000 | 0.0000 | 0.0000 |
| 1.00 | 0.0005 | 0.0000 | 0.0000 | 0.0000 | 0.0000 | 0.0000 |
| 1.20 | 0.0021 | 0.0001 | 0.0000 | 0.0000 | 0.0000 | 0.0000 |
| 1.40 | 0.0053 | 0.0002 | 0.0000 | 0.0000 | 0.0001 | 0.0000 |
| 1.60 | 0.0136 | 0.0007 | 0.0003 | 0.0001 | 0.0000 | 0.0000 |
| 1.80 | 0.0347 | 0.0022 | 0.0007 | 0.0002 | 0.0000 | 0.0001 |
| 2.00 | 0.1026 | 0.0071 | 0.0018 | 0.0003 | 0.0001 | 0.0000 |
| 2.20 | 0.2202 | 0.0158 | 0.0040 | 0.0005 | 0.0002 | 0.0001 |
| 2.40 | 0.4449 | 0.0359 | 0.0103 | 0.0012 | 0.0004 | 0.0003 |
| 2.60 | 0.7000 | 0.0821 | 0.0212 | 0.0026 | 0.0009 | 0.0004 |
| 2.80 | 0.8965 | 0.1630 | 0.0441 | 0.0065 | 0.0018 | 0.0009 |
| 3.00 | 0.9777 | 0.2728 | 0.0836 | 0.0083 | 0.0028 | 0.0016 |
| 3.20 | 0.9973 | 0.4542 | 0.1525 | 0.0171 | 0.0066 | 0.0027 |
| 3.40 | 0.9999 | 0.6233 | 0.2441 | 0.0306 | 0.0097 | 0.0057 |
| 3.60 | 1.0000 | 0.7775 | 0.3613 | 0.0476 | 0.0155 | 0.0076 |
| 3.80 | 1.0000 | 0.8883 | 0.5218 | 0.0830 | 0.0277 | 0.0133 |
| 4.00 | | 0.9593 | 0.6743 | 0.1199 | 0.0454 | 0.0235 |
| 4.20 | | 0.9905 | 0.7990 | 0.1903 | 0.0732 | 0.0343 |
| 4.40 | | 0.9980 | 0.8912 | 0.2637 | 0.1055 | 0.0557 |
| 4.60 | | 0.9996 | 0.9468 | 0.3732 | 0.1551 | 0.0827 |
| 4.80 | | 1.0000 | 0.9790 | 0.4852 | 0.2181 | 0.1084 |
| 5.00 | | 1.0000 | 0.9944 | 0.6052 | 0.2920 | 0.1629 |
| 5.20 | | | 0.9983 | 0.7020 | 0.3768 | 0.2199 |
| 5.40 | | | 0.9998 | 0.7969 | 0.4713 | 0.2844 |
| 5.60 | | | 0.9999 | 0.8692 | 0.5777 | 0.3726 |
| 5.80 | | | 1.0000 | 0.9283 | 0.6727 | 0.4564 |
| 6.00 | | | | 0.9591 | 0.7660 | 0.5478 |
| 6.20 | | | | 0.9843 | 0.8363 | 0.6283 |
| 6.40 | | | | 0.9919 | 0.8999 | 0.7265 |
| 6.60 | | | | 0.9980 | 0.9325 | 0.8067 |
| 6.80 | | | | 0.9990 | 0.9653 | 0.8573 |
| 7.00 | | | | 0.9998 | 0.9818 | 0.9068 |
| 7.20 | | | | 1.0000 | 0.9906 | 0.9438 |
| 7.40 | | | | 1.0000 | 0.9968 | 0.9683 |
| 7.60 | | | | 1.0000 | 0.9985 | 0.9830 |
| 7.80 | | | | 1.0000 | 0.9994 | 0.9915 |
| 8.00 | | | | | 0.9997 | 0.9956 |
| 8.20 | | | | | 0.9999 | 0.9982 |
| 8.40 | | | | | 1.0000 | 0.9992 |
| 8.60 | | | | | | 0.9998 |
| 8.80 | | | | | | 0.9999 |
| 9.00 | | | | | | 1.0000 |
| 9.20 | | | | | | 1.0000 |


[3] Bannerman, M. N.; Sargant, R.; Lue, L. DynamO: A Free O(N) General Event-Driven Molecular Dynamics Simulator. *J. Comput. Chem.* **2011**, *32*, 3329-3338.

[4] Lubachevsky, B. D.; Stillinger, F. H. Geometric Properties of Random Disk Packings. *J. Stat. Phys.* **1990**, *60*, 561-583.

[5] Baranau, V.; Tallarek, U. Random-Close Packing Limits for Monodisperse and Polydisperse Hard Spheres. *Soft Matter* **2014**, *10*, 3826-3841.

[6] Lazar, E. A. VoroTop: Voronoi Cell Topology Visualization and Analysis Toolkit. *Modell. Simul. Mater. Sci. Eng.* **2017**, *26*, 015011.

[7] Tutte, W. T. How to Draw a Graph. *Proc. London Math. Soc.* **1963**, *3*, 743-767.

[8] Stoll, E. A Fast Cluster Counting Algorithm for Percolation On and Off Lattices. *Comput. Phys. Commun.* **1998**, *109*, 1-5.

[9] Stauffer, D.; Aharony, A. *Introduction to Percolation Theory*; Taylor & Francis: London, 1994.

[10] Jerauld, G. R.; Scriven, L. E.; Davis, H. T. Percolation and Conduction on the 3D Voronoi and Regular Networks: a Second Case Study in Topological Disorder. *J. Phys. C* **1984**, *17*, 3429.

[11] Lazar, E. A.; Mason, J. K.; MacPherson, R. D.; Srolovitz, D. J. Statistical Topology of Three-Dimensional Poisson-Voronoi Cells and Cell Boundary Networks *Phys. Rev. E* **2013**, *88*, 063309.

TABLE S3. Voronoi cell types observed in the ideal gas. Most of the scarcely observed Weinberg vectors in the ideal gas were not discovered in the maximally random jammed state.

| Number | Rank | Weinberg vector | $f_{id}$ [%] |
|---|---|---|---|
| 1 | 1 | (1,2,3,1,3,4,5,6,1,6,7,8,9,2,9,10,11,4,11,12,5,12,13,7,13,14,8,14,10,14,13,12,11,10,9,8,7, $\cdots$ | 0.273956 |
| 2 | 2 | (1,2,3,1,3,4,5,6,1,6,7,8,2,8,9,10,4,10,11,5,11,12,7,12,9,12,11,10,9,8,7,6,5,4,3,2,1) $\cdots$ | 0.166280 |
| 3 | 3 | (1,2,3,4,1,4,5,6,1,6,7,8,9,2,9,10,11,3,11,12,13,5,13,14,7,14,15,8,15,16,10,16,12,16,15,14, $\cdots$ | 0.158408 |
| 4 | 4 | (1,2,3,1,3,4,5,6,1,6,7,8,9,2,9,10,11,12,4,12,13,5,13,14,7,14,15,16,8,16,10,16,15,11,15,14, $\cdots$ | 0.119908 |
| 5 | 5 | (1,2,3,4,1,4,5,6,1,6,7,8,2,8,9,10,3,10,11,12,5,12,13,7,13,14,9,14,11,14,13,12,11,10,9,8,7, $\cdots$ | 0.116908 |
| 6 | 6 | (1,2,3,4,1,4,5,6,1,6,7,8,2,8,9,10,3,10,11,5,11,12,7,12,9,12,11,10,9,8,7,6,5,4,3,2,1) $\cdots$ | 0.101192 |
| 7 | 7 | (1,2,3,1,3,4,5,6,1,6,7,8,9,2,9,10,11,12,4,12,13,5,13,14,15,7,15,16,8,16,10,16,15,14,11,14, $\cdots$ | 0.096052 |
| 8 | 8 | (1,2,3,1,3,4,5,6,7,1,7,8,9,10,2,10,11,12,13,4,13,14,5,14,15,16,6,16,8,16,15,17,18,9,18,11, $\cdots$ | 0.094484 |
| 9 | 9 | (1,2,3,4,1,4,5,6,7,1,7,8,9,2,9,10,11,3,11,12,13,5,13,14,6,14,15,16,8,16,17,10,17,18,12,18, $\cdots$ | 0.094280 |
| 10 | 10 | (1,2,3,1,3,4,5,6,1,6,7,8,9,2,9,10,11,4,11,12,5,12,13,14,7,14,15,8,15,16,10,16,13,16,15,14, $\cdots$ | 0.093932 |
| 11 | 11 | (1,2,3,4,1,4,5,6,1,6,7,8,2,8,9,10,11,3,11,12,13,5,13,14,15,7,15,16,9,16,17,10,17,18,12,18, $\cdots$ | 0.093804 |
| 12 | 12 | (1,2,3,1,3,4,5,6,1,6,7,8,9,2,9,10,11,12,4,12,13,14,5,14,7,14,13,15,16,8,16,10,16,15,11,15, $\cdots$ | 0.093764 |
| 13 | 13 | (1,2,3,4,1,4,5,6,1,6,7,8,2,8,9,10,3,10,11,12,5,12,13,14,7,14,15,9,15,16,11,16,13,16,15,14, $\cdots$ | 0.091052 |
| 14 | 14 | (1,2,3,1,3,4,5,6,1,6,7,8,2,8,9,10,4,10,11,12,5,12,13,7,13,14,9,14,11,14,13,12,11,10,9,8,7, $\cdots$ | 0.090872 |
| 15 | 15 | (1,2,3,4,1,4,5,6,1,6,7,8,2,8,9,10,11,3,11,12,5,12,13,14,7,14,9,14,13,10,13,12,11,10,9,8,7, $\cdots$ | 0.089296 |
| 16 | 16 | (1,2,3,1,3,4,5,6,1,6,7,8,9,2,9,10,11,4,11,12,13,5,13,14,7,14,15,16,8,16,10,16,15,12,15,14, $\cdots$ | 0.088040 |
| 17 | 17 | (1,2,3,1,3,4,5,6,1,6,7,8,9,2,9,10,11,12,4,12,13,14,5,14,15,7,15,16,17,8,17,10,17,16,18,11, $\cdots$ | 0.083204 |
| 18 | 18 | (1,2,3,1,3,4,5,6,1,6,7,8,9,2,9,10,11,4,11,12,13,5,13,14,7,14,15,8,15,16,10,16,12,16,15,14, $\cdots$ | 0.082168 |
| 19 | 19 | (1,2,3,1,3,4,5,6,1,6,7,8,9,2,9,10,11,12,4,12,13,14,5,14,15,7,15,16,11,16,13,16,15,14,13,12 $\cdots$ | 0.081084 |
| 20 | 20 | (1,2,3,1,3,4,5,6,1,6,7,8,9,2,9,10,11,12,4,12,13,5,13,14,7,14,11,14,13,12,11,10,8,10,9,8,7, $\cdots$ | 0.080248 |
| 21 | 21 | (1,2,3,4,1,4,5,6,7,1,7,8,9,2,9,10,11,3,11,12,13,5,13,14,6,14,15,8,15,16,10,16,12,16,15,14, $\cdots$ | 0.078672 |
| 22 | 22 | (1,2,3,1,3,4,5,6,7,1,7,8,9,10,2,10,11,12,4,12,13,5,13,14,6,14,15,8,15,16,9,16,11,16,15,14, $\cdots$ | 0.077020 |
| 23 | 23 | (1,2,3,4,1,4,5,6,1,6,7,8,9,2,9,10,11,3,11,12,13,5,13,14,15,7,15,16,8,16,17,10,17,18,12,18, $\cdots$ | 0.075512 |
| 24 | 24 | (1,2,3,1,3,4,5,6,1,6,7,8,9,10,2,10,11,12,13,4,13,14,5,14,15,16,7,16,8,16,15,12,15,14,13,12 $\cdots$ | 0.071504 |
| $\vdots$ | | | |
| 9,710,780 | 1,453,499 | (1,2,3,1,3,4,5,1,5,6,7,2,7,8,9,10,4,10,11,12,13,14,6,14,15,16,17,8,17,18,9,18,16,18,17,16, $\cdots$ | 0.000004 |

TABLE S4. Voronoi cell types observed in the maximally random jammed state. The total number of the types were . Most of the Weinberg vectors in the maximally random jammed state were included in those of the ideal gas.

| Number | Rank | Weinberg vector | $f_{mrj}$ [%] |
|---|---|---|---|
| 1 | 1 | (1,2,3,4,1,4,5,6,7,1,7,8,9,10,2,10,11,12,3,12,13,14,5,14,15,16,6,16,17,8,17,18,19,9,19,20, $\cdots$ | 3.485016 |
| 2 | 2 | (1,2,3,4,1,4,5,6,7,1,7,8,9,2,9,10,11,12,3,12,13,14,5,14,15,16,6,16,17,18,8,18,19,10,19,20, $\cdots$ | 2.401300 |
| 3 | 3 | (1,2,3,4,1,4,5,6,7,1,7,8,9,2,9,10,11,12,3,12,13,14,5,14,15,16,6,16,17,18,8,18,19,20,10,20, $\cdots$ | 2.058644 |
| 4 | 4 | (1,2,3,4,1,4,5,6,7,1,7,8,9,10,2,10,11,12,13,3,13,14,15,5,15,16,17,6,17,18,8,18,19,20,9,20, $\cdots$ | 1.760012 |
| 5 | 5 | (1,2,3,4,1,4,5,6,7,1,7,8,9,10,2,10,11,12,13,3,13,14,15,5,15,16,17,6,17,18,8,18,19,20,9,20, $\cdots$ | 1.556520 |
| 6 | 6 | (1,2,3,4,1,4,5,6,7,1,7,8,9,2,9,10,11,12,3,12,13,14,5,14,15,16,6,16,17,18,8,18,19,10,19,20, $\cdots$ | 1.510904 |
| 7 | 7 | (1,2,3,4,1,4,5,6,7,1,7,8,9,2,9,10,11,12,3,12,13,14,5,14,15,16,6,16,17,8,17,18,10,18,19,20, $\cdots$ | 1.508568 |
| 8 | 8 | (1,2,3,4,1,4,5,6,7,1,7,8,9,10,2,10,11,12,3,12,13,14,5,14,15,16,6,16,17,18,8,18,19,9,19,20, $\cdots$ | 1.468844 |
| 9 | 9 | (1,2,3,4,5,1,5,6,7,8,1,8,9,10,2,10,11,12,3,12,13,14,4,14,15,6,15,16,17,7,17,18,9,18,19,11, $\cdots$ | 1.365496 |
| 10 | 10 | (1,2,3,1,3,4,5,6,7,1,7,8,9,10,2,10,11,12,4,12,13,14,5,14,15,16,6,16,17,8,17,18,19,9,19,20, $\cdots$ | 1.272144 |
| 11 | 11 | (1,2,3,4,1,4,5,6,7,1,7,8,9,2,9,10,11,12,3,12,13,14,5,14,15,16,6,16,17,8,17,18,19,10,19,20, $\cdots$ | 1.245668 |
| 12 | 12 | (1,2,3,1,3,4,5,6,7,1,7,8,9,10,2,10,11,12,13,4,13,14,5,14,15,16,6,16,17,8,17,18,19,9,19,20, $\cdots$ | 0.956396 |
| 13 | 13 | (1,2,3,1,3,4,5,6,7,1,7,8,9,10,2,10,11,12,13,4,13,14,15,5,15,16,17,6,17,18,8,18,19,20,9,20, $\cdots$ | 0.828632 |
| 14 | 14 | (1,2,3,1,3,4,5,6,7,1,7,8,9,10,2,10,11,12,13,4,13,14,5,14,15,16,17,6,17,18,8,18,19,20,9,20, $\cdots$ | 0.808980 |
| 15 | 15 | (1,2,3,4,1,4,5,6,7,1,7,8,9,2,9,10,11,12,3,12,13,14,5,14,15,16,6,16,17,8,17,18,19,10,19,20, $\cdots$ | 0.760416 |
| 16 | 16 | (1,2,3,4,1,4,5,6,7,1,7,8,9,10,2,10,11,12,13,3,13,14,15,5,15,16,17,6,17,18,8,18,19,20,21,9, $\cdots$ | 0.736144 |
| 17 | 17 | (1,2,3,4,1,4,5,6,7,1,7,8,9,2,9,10,11,12,3,12,13,14,5,14,15,16,6,16,17,18,8,18,19,10,19,20, $\cdots$ | 0.708408 |
| 18 | 18 | (1,2,3,4,1,4,5,6,7,1,7,8,9,10,2,10,11,12,3,12,13,14,5,14,15,16,6,16,17,18,8,18,19,9,19,20, $\cdots$ | 0.704128 |
| 19 | 19 | (1,2,3,4,1,4,5,6,7,1,7,8,9,2,9,10,11,12,3,12,13,14,5,14,15,16,17,6,17,18,8,18,19,20,10,20, $\cdots$ | 0.695412 |
| 20 | 20 | (1,2,3,4,1,4,5,6,7,1,7,8,9,10,2,10,11,12,3,12,13,14,5,14,15,16,6,16,17,8,17,18,19,9,19,20, $\cdots$ | 0.686692 |
| 21 | 21 | (1,2,3,4,1,4,5,6,7,1,7,8,9,10,2,10,11,12,13,3,13,14,15,5,15,16,17,6,17,18,19,8,19,20,9,20, $\cdots$ | 0.680040 |
| 22 | 22 | (1,2,3,4,1,4,5,6,7,1,7,8,9,2,9,10,11,3,11,12,13,5,13,14,15,6,15,16,17,8,17,18,19,10,19,20, $\cdots$ | 0.633432 |
| 23 | 23 | (1,2,3,1,3,4,5,6,7,1,7,8,9,10,2,10,11,12,13,4,13,14,5,14,15,16,17,6,17,18,8,18,19,20,9,20, $\cdots$ | 0.604276 |
| 24 | 24 | (1,2,3,4,1,4,5,6,7,1,7,8,9,10,2,10,11,12,13,3,13,14,15,5,15,16,17,6,17,18,19,8,19,20,9,20, $\cdots$ | 0.587344 |
| $\vdots$ | | | |
| 325,399 | 158,644 | (1,2,3,4,5,1,5,6,7,8,1,8,9,10,2,10,11,12,3,12,13,14,15,4,15,16,17,6,17,18,19,7,19,20,21,9, $\cdots$ | 0.000004 |

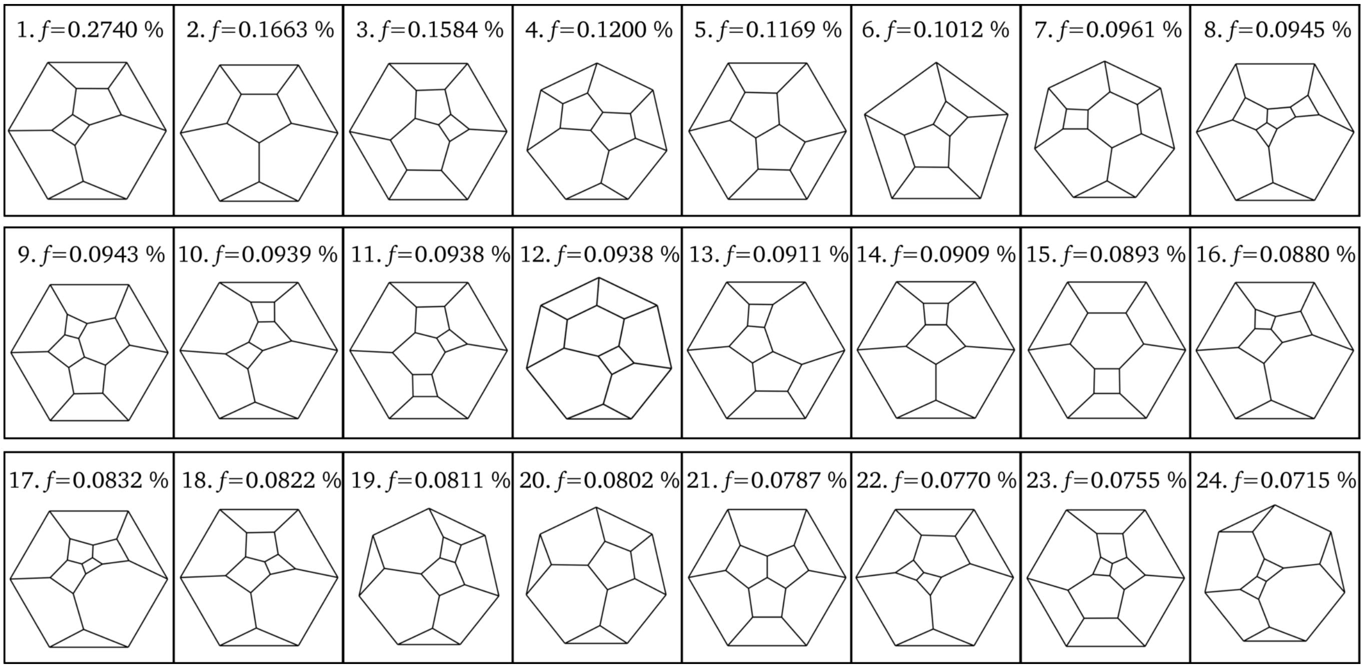


FIG. S3. Schlegel diagrams of the 24 most common topological types among the cells observed in the ideal gas. The list of the frequently observed Weinberg vectors is almost identical with that obtained by Lazar et al.[11].

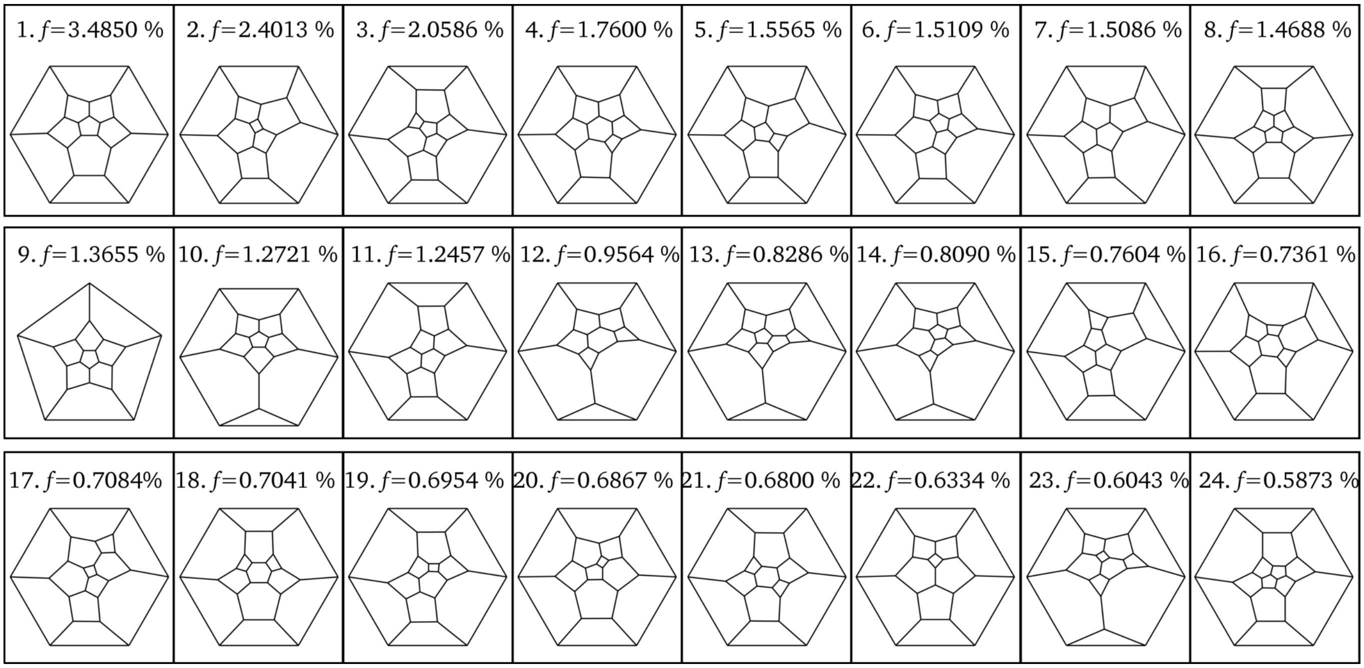


FIG. S4. Schlegel diagrams of the 24 most common topological types among the cells observed in the maximally random jammed state. Compared to the list of the Weinberg vectors of the ideal gas, the frequently observed types of the Voronoi cells in the maximally random jammed state are more symmetric.
